# Supplementary material for: Faster No-Regret Learning Dynamics for Extensive-Form Correlated and Coarse Correlated Equilibria
Source: arXiv:2202.05446 source file (2022-02-11)
Supplement: Supplementary file 1 [file appendix_related_work.tex]

\section{Additional Related Work}
